# Supplementary material for: In memoriam Leonid V. Keldysh
Source: arXiv:1901.01065 source file (2019-01-04)
Supplement: Supplementary file 3 [file test2.tex]

%% test2.tex
%%
%% This is file `test2.tex', one of a set of several test/example files
%% in the `subfig' package.
%%
%% Copyright © 2003, 2004, 2005 Steven Douglas Cochran.
%% 
%% This work (the subfig package) may be distributed and/or modified 
%% under the conditions of the LaTeX Project Public License, either 
%% version 1.3 of this license or (at your option) any later version.
%% The latest version of this license is in
%%   http://www.latex-project.org/lppl.txt
%% and version 1.3 or later is part of all distributions of LaTeX
%% version 2003/12/01 or later.
%%
%% This work has the LPPL maintenance status "author-maintained".
%% 
%% This Current Maintainer of this work is Steven Douglas Cochran.
%%
%% This work consists of all files listed under "MANIFEST" in the
%% README file distributed with the subfig package.

\documentclass{article}

\usepackage{fullpage}
\usepackage[format=hang]{subfig}
\captionsetup[subfloat]{farskip=7pt,nearskip=3pt}

\makeatletter
  \def\mpt{\@minipagetrue}
  \def\mpf{\@minipagefalse}
  \renewcommand\abstract[1]{%
    \def\@abstract{%
      \centerline{{\large\bf Abstract}}
      \noindent
      #1}}
  \renewcommand\@maketitle{%
    \newpage
    \null\vfil
    \vskip 60\p@
    \begin{center}%
      {\LARGE \@title \par}%
      \vskip 3em%
      {\large
       \lineskip .75em%
       \begin{tabular}[t]{c}%
         \@author
       \end{tabular}\par}%
      \vskip 1.5em%
      {\large \@date \par}% 
    \end{center}%
    \vskip 2.5em%
    \@abstract
    \vfil\null}%
\makeatother

\fboxsep=-\fboxrule
\newcommand{\figbox}[1]{%
  \fbox{%
    \vbox to 1in{%
    \vfil
    \hbox to 2in{%
      \hfil
      #1%
      \hfil}%
    \vfil}}}
\def\hrl{\hbox to 0pt{\hss\vrule height0pt depth.2pt width9.5pt}}
\def\hrr{\hbox to 0pt{\vrule height0pt depth.2pt width9.5pt\hss}}

\begin{document}

\title{Subfig Package Test Program Two}
\author{Steven Douglas Cochran\\
        Digital Mapping Laboratory\\
        School of Computer Science\\
        Carnegie-Mellon University\\
        5000 Forbes Avenue\\
        Pittsburgh, PA 15213-3890\\
        USA}
\date{21 December 2003}
\abstract{%
This test checks three things:
\begin{enumerate}
  \item subfloat references; 
  \item subfloat options; and,
  \item extra blank space in the caption layout.
\end{enumerate}}
\maketitle
\clearpage

Figures wrapped to show any extra spaces introduced in processing the
sub-floats.

\begin{figure}%
  \centering
  \fbox{%
    \fbox{\subfloat[Subfigure One.\label{fig:A1}]{%
      \figbox{SUBFIG ONE}}}%
    \hspace{10pt}%
    \fbox{\subfloat[Subfigure Two.\label{fig:A2}]{%
      \figbox{SUBFIG TWO}}}}
  \caption{Two side-by-side figures.}%
  \label{fig:A}%
\end{figure}

\begin{figure}%
  \begin{center}%
    \fbox{\hbox to 4.13837in{\hss\vbox{%
      \fbox{\mpt\subfloat[Subfigure Three.\label{fig:B1}]{%
        \figbox{SUBFIG THREE}}}%
      \hspace{10pt}%
      \fbox{\mpt\subfloat[Subfigure Four.\label{fig:B2}]{%
        \figbox{SUBFIG FOUR}}}\\[-1.5pt]
      \fbox{\subfloat[Subfigure Five.\label{fig:B3}]{%
        \figbox{SUBFIG FIVE}}}%
      \hspace{10pt}%
      \fbox{\subfloat[Subfigure Six.\label{fig:B4}]{%
        \figbox{SUBFIG SIX}}}}\hss}}%
    \end{center}
  \caption{Four figures with specified suppression of extra padding.}%
  \label{fig:B}%
\end{figure}

\begin{figure}
  \centering
  \fbox{%
    \begin{minipage}{4.13837in}%
%\mpf
      \subfloat[Subfigure Seven.\label{fig:C1}]{%
        \figbox{SUBFIG SEVEN}}
      \hspace{10pt}%
      \subfloat[Subfigure Eight.\label{fig:C2}]{%
      \figbox{SUBFIG EIGHT}}\\
      \subfloat[Subfigure Nine.\label{fig:C3}]{%
        \figbox{SUBFIG NINE}}
      \hspace{10pt}%
      \subfloat[Subfigure Ten.\label{fig:C4}]{%
        \figbox{SUBFIG TEN}}
    \end{minipage}}
    \caption{Four figures with auto fitting in a minipage.}%
    \label{fig:C}%
\end{figure}

\begin{figure}
  \centering
%
  \subfloat[First caption.]{\fbox{Under figure/text}}\quad
  \subfloat[Longer second caption.]{\fbox{Under figure/text}}\\
%
  \subfloat[Third caption.]{\figbox{Under figure/text}}\quad
  \subfloat[Longer fourth caption. longer fourth caption.
             longer fourth caption.]{\figbox{Under figure/text}}
  \caption{Four figures testing caption fitting.}%
\end{figure}


\newpage

\begin{table}
  \centering
%
  \caption{Test for TABTOPCAP with caption.}%
%
  \leavevmode\vtop{\vbox{\hbox to .5in{\hfil TEST\hrr}}\vbox{\hbox to .5in{\hfil Box}}}\quad
  \subfloat[First caption.]{\figbox{Table A with caption}}\quad
  \subfloat[Second caption.]{\figbox{Table B with caption}}\quad
  \vtop{\vbox{\hbox to .5in{\hrl TEST\hfil}}\vbox{\hbox to .5in{Box\hfil}}}\\
%
  \leavevmode\vtop{\vbox{\hbox to .5in{\hfil TEST\hrr}}\vbox{\hbox to .5in{\hfil Box}}}\quad
  \subfloat[Third caption.]{\figbox{Table C with caption}}\quad
  \subfloat[Longer fourth caption. longer fourth caption.
            longer fourth caption.]{\figbox{Table D with caption}}\quad
  \vtop{\vbox{\hbox to .5in{\hrl TEST\hfil}}\vbox{\hbox to .5in{Box\hfil}}}
%
\end{table}

\begin{table}
  \centering
%
  \caption{Test for TABTOPCAP without caption.}%
%
  \leavevmode\vtop{\vbox{\hbox to .5in{\hfil TEST\hrr}}\vbox{\hbox to .5in{\hfil Box}}}\quad
  \subfloat{\figbox{Table A with/out caption}}\quad
  \subfloat[Second caption.]{\figbox{Table B with caption}}\quad
  \vtop{\vbox{\hbox to .5in{\hrl TEST\hfil}}\vbox{\hbox to .5in{Box\hfil}}}\\
%

  \leavevmode\vtop{\vbox{\hbox to .5in{\hfil TEST\hrr}}\vbox{\hbox to .5in{\hfil Box}}}\quad
  \subfloat{\figbox{Table C with/out caption}}\quad
  \subfloat[Longer fourth caption. longer fourth caption.
            longer fourth caption.]{\figbox{Table D with caption}}\quad
  \vtop{\vbox{\hbox to .5in{\hrl TEST\hfil}}\vbox{\hbox to .5in{Box\hfil}}}
%
\end{table}




\end{document}
